# Supplementary material for: Evaluating Adversarial Robustness with Expected Viable Performance
Source: arXiv:2309.09928 source file (2023-09-18)
Supplement: Supplementary file 1 [file appendix.tex]

\subsection{Convergence of Trapezoid Approximation}
%In Figure~\ref{fig:cifar}, the adversarial trained model at 0.5 $L_2$ distance receives a higher EVP than the model trained at 1.0 $L_2$ distance.
%This is a notable distinction between our definition of robustness and the robustness induced at higher levels of adversarial training. 
%In our metric, any region in the perturbation space where performance is below the viable threshold is considered non-functional and is not counted in the robustness evaluation.
%Despite the entirety of the area under the curve being larger, the model acting in a region below the threshold would not be selected for a given application.
An important part of any metric is that it converges to a single value given greater levels of precision. 
We demonstrate via experiments that EVP converges with more sampling intervals in the perturbation space.
In Fig.~\ref{fig:convergence}, finer intervals of the perturbation space allow for more precision in measuring EVP. 
One caveat to the measurement is understanding that the interval can only be as fine grained as the attack itself. 
A PGD step size must be less than the sampling interval. 
Using smaller intervals requires more adversarially attacked images to be computed for each interval, increasing the data storage and training time requirements. 
It is recommended to use an interval size of less than or equal to 0.1 $L_2$ distance. 
The PGD step size for Fig.~\ref{fig:convergence} is $step=0.005$ for all trials.

\begin{figure}[ht]
  \centering
  \includegraphics[width=8cm]{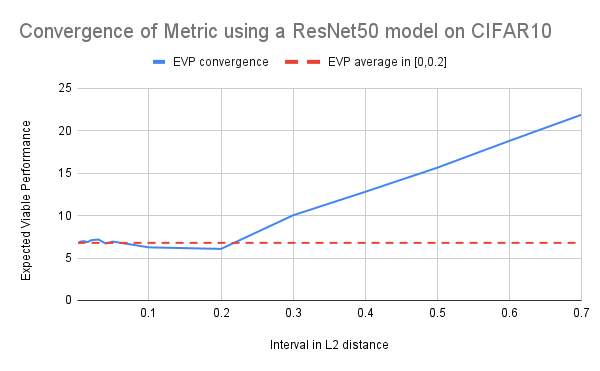}
  \caption{Selecting the interval size in the perturbation space is stable at $\Delta\epsilon < 0.2$ in $L_2$ distance.}
\label{fig:convergence}
\end{figure}

\subsection{Approximate Calculation Alternative}
The perturbation space can be sampled in given intervals through bounding adversarial sample generation to given $L_2$ distances from original samples. 
By generating a set of test images within some perturbation interval $\epsilon_i$, the whole perturbation space can be denoted by $E$ (for environment) as ${\epsilon_0, \epsilon_1, ..., \epsilon_i, ..., \epsilon_n} \equiv E$. 
Samples are selected at each interval sufficiently close to but not passing the bound $\sup \epsilon_i$, which is known as the perturbation budget or perturbation bound.
Performance (here, accuracy) can then be measured over the perturbed dataset at each increment on the perturbation scale. 
The probability of a sample falling into any given perturbation region is measured by the size of the region. 
This metric can be summarized in the following equation where $|\epsilon_i| = \sup \epsilon_i - \inf \epsilon_i$,

\[ R_\tau(s) = \sum_{\epsilon_i \subset E}^{} a(s,\epsilon_i) * |\epsilon_i| \]

However, the idea of maintaining functionality to be robust requires defining a minimum performance threshold for functionality in the context of a given application. 
This value is application dependent and may be determined given the risks and specific environmental variabilities in which a system is to operate. 
Let $\tau$ be the functional threshold. 
The robust region $R(s) = \{\epsilon_i  |  a(s,\epsilon_i) \geq \tau\}$ is the subset of the perturbation space where the model maintains functionality.
Robustness is then written as,
\[ R_\tau(s) = \sum_{\epsilon_i \subset E}^{} a(s,\epsilon_i) * \mathds{1}[a(s,\epsilon_i) \geq \tau] * |\epsilon_i| \]

For adversarial generation of perturbations relying on a perturbation budget, the actual perturbation magnitudes may be less than the corresponding budget, and the expected value is interpreted with respect to a distribution over budgets rather than directly over perturbation sizes. 
For better precision, the $\epsilon_i$ cuts need not be taken at equal intervals but can instead be denser in regions where accuracy is changing more rapidly, as well as where it is near the chosen threshold $\tau$.
\[ R_\tau(s) = \sum_{\epsilon_i \subset R}^{} a(s,\epsilon_i) * |\epsilon_i| \]

\subsection{$L_\infty$ Examples}
The following figures show the metric applied to $L_\infty$ PGD perturbations.
\begin{figure}[ht]
    \centering
    \includegraphics[width=8cm]{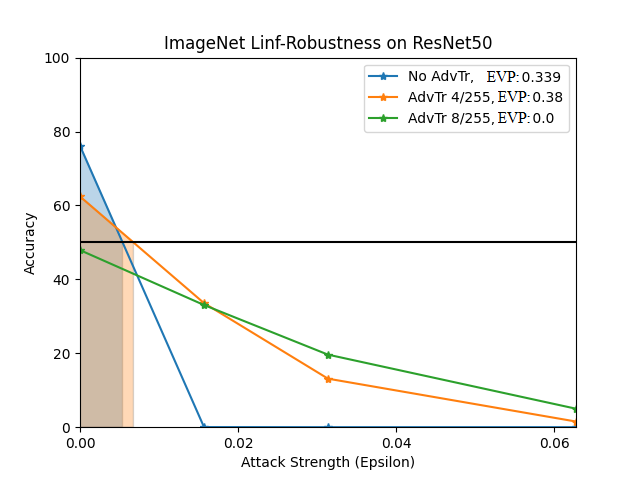}
    \caption{Our approach on an ImageNet model. Each $L_\infty$ value is reported over 255. $\tau=50\%$}
  \label{fig:imagenetinf}
  \end{figure}

  \begin{figure}[ht]
    \centering
    \includegraphics[width=8cm]{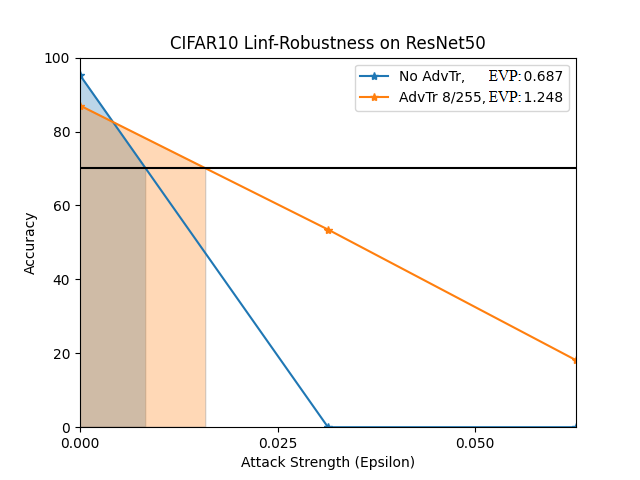}
    \caption{Our approach on a CIFAR model. Each $L_\infty$ value is reported over 255. $\tau=70\%$}
  \label{fig:cifarinf}
  \end{figure}
